# Supplementary material for: Z-SASLM: Zero-Shot Style-Aligned SLI Blending Latent Manipulation
Source: arXiv:2503.23234 source file (2025-03-29)
Supplement: Supplementary file 1 [file X_suppl.tex]

\clearpage
\setcounter{page}{1}
\maketitlesupplementary

\section{\textbf{Music2Text: Query List}}
\label{appendix:music2text_query_list}

In this section, we present the list of predefined textual queries used in the Music2Text component of our multi-modal fusion pipeline. These queries capture various moods, atmospheres, and tonal qualities of music, allowing for a comprehensive interpretation of the audio content in the image generation process.

\begin{itemize}
    \item \textit{"dark and intense"}
    \item \textit{"bright and energetic"}
    \item \textit{"calm and peaceful"}
    \item \textit{"gritty and rebellious"}
    \item \textit{"ethereal and dreamy"}
    \item \textit{"mysterious and shadowy"}
    \item \textit{"uplifting and inspirational"}
    \item \textit{"melancholic and deep"}
    \item \textit{"joyful and vibrant"}
    \item \textit{"nostalgic and warm"}
    \item \textit{"soft and serene"}
    \item \textit{"fast and aggressive"}
    \item \textit{"slow and emotional"}
    \item \textit{"expansive and cinematic"}
    \item \textit{"mechanical and futuristic"}
    \item \textit{"natural and organic"}
    \item \textit{"chaotic and energetic"}
    \item \textit{"minimalist and clean"}
    \item \textit{"heavy and thunderous"}
    \item \textit{"grand and majestic"}
    \item \textit{"smooth and jazzy"}
    \item \textit{"vibrant and colorful"}
    \item \textit{"subdued and introspective"}
    \item \textit{"intense and fiery"}
\end{itemize}

\section{\textbf{Linear vs SLI Interpolation: Theoretical Deepening}}
\label{appendix:linear_vs_slerp_theory}

From the results in Table \ref{tab:weighted_dino_comparison}, we observed that while linear interpolation may appear straightforward for blending styles, it has notable drawbacks in non-linear latent spaces, such as those found in text-to-image models like Stable Diffusion. SLI, on the other hand, provides a more geometrically consistent approach. We detail the differences below:

\begin{itemize}

    \item \textbf{Latent Space Curvature}: The latent space in generative models is typically non-linear and lies on a complex, curved manifold. This means that the vectors representing different styles do not exist in a flat, Euclidean space but instead are positioned on the surface of a high-dimensional hypersphere. Indeed, when applying linear interpolation between two or more latent vectors in a non-linear latent space, the result may not lie in the meaningful regions of the latent space. Specifically, linear interpolation computes the weighted average of vectors without considering the curvature of the space. This can cause the interpolated vector to "fall off" the manifold, meaning the generated image may lack coherence or exhibit visual artifacts. On the other hand, SLI, by definition, interpolates along the surface of the hypersphere, preserving the non-linear geometry of the latent space. By moving along the shortest path (a.k.a. geodesic) between two points on the hypersphere, SLI ensures that the resulting latent vector remains in a geometrically consistent and meaningful region of the latent space. This makes SLI a far better option when working with generative models that operate in non-linear latent spaces.
    
    \item \textbf{Feature and Detail Preservation}: While linear interpolation averages style vectors without accounting for the underlying curvature of the latent space, it often results in a blended vector biased toward one style, potentially losing distinct stylistic features. This leads to a "compromise" vector, causing blurring and a lack of coherent stylistic details. SLI, in contrast, respects the geometric properties of the latent space by interpolating along the hypersphere. It smoothly integrates features from both styles, preserving the key elements such as color palettes, and textures, resulting in a more balanced and visually coherent blend. This ensures that each style features are balanced in the generated images, without having any of the style to be over-represented or under-represented.

    \item \textbf{Multi-Dimensional Consistency}: When blending more than two styles, the challenge becomes even more pronounced as the number of latent vectors increases. Ensuring consistency across multiple styles requires a method that can handle multi-dimensional latent spaces effectively. Linear Interpolation may fail to account for the complexities of multi-dimensional latent spaces, especially when blending more than two styles. The lack of geometric consistency in the blending process can result in an intermediate vector that is far removed from the actual manifold where meaningful representations of styles lie. SLI, on the other hand, can be extended recursively to handle multiple styles. By applying SLI pairwise across all style vectors and ensuring that the resulting blended vector remains on the hypersphere, SLI preserves multi-dimensional consistency. This means that even as more styles are introduced, the blending remains smooth and coherent, and the final latent vector continues to respect the non-linear structure of the latent space.

\end{itemize}

\begin{figure*}[ht]
    \centering
    % First full-width image
    \includegraphics[width=\linewidth]{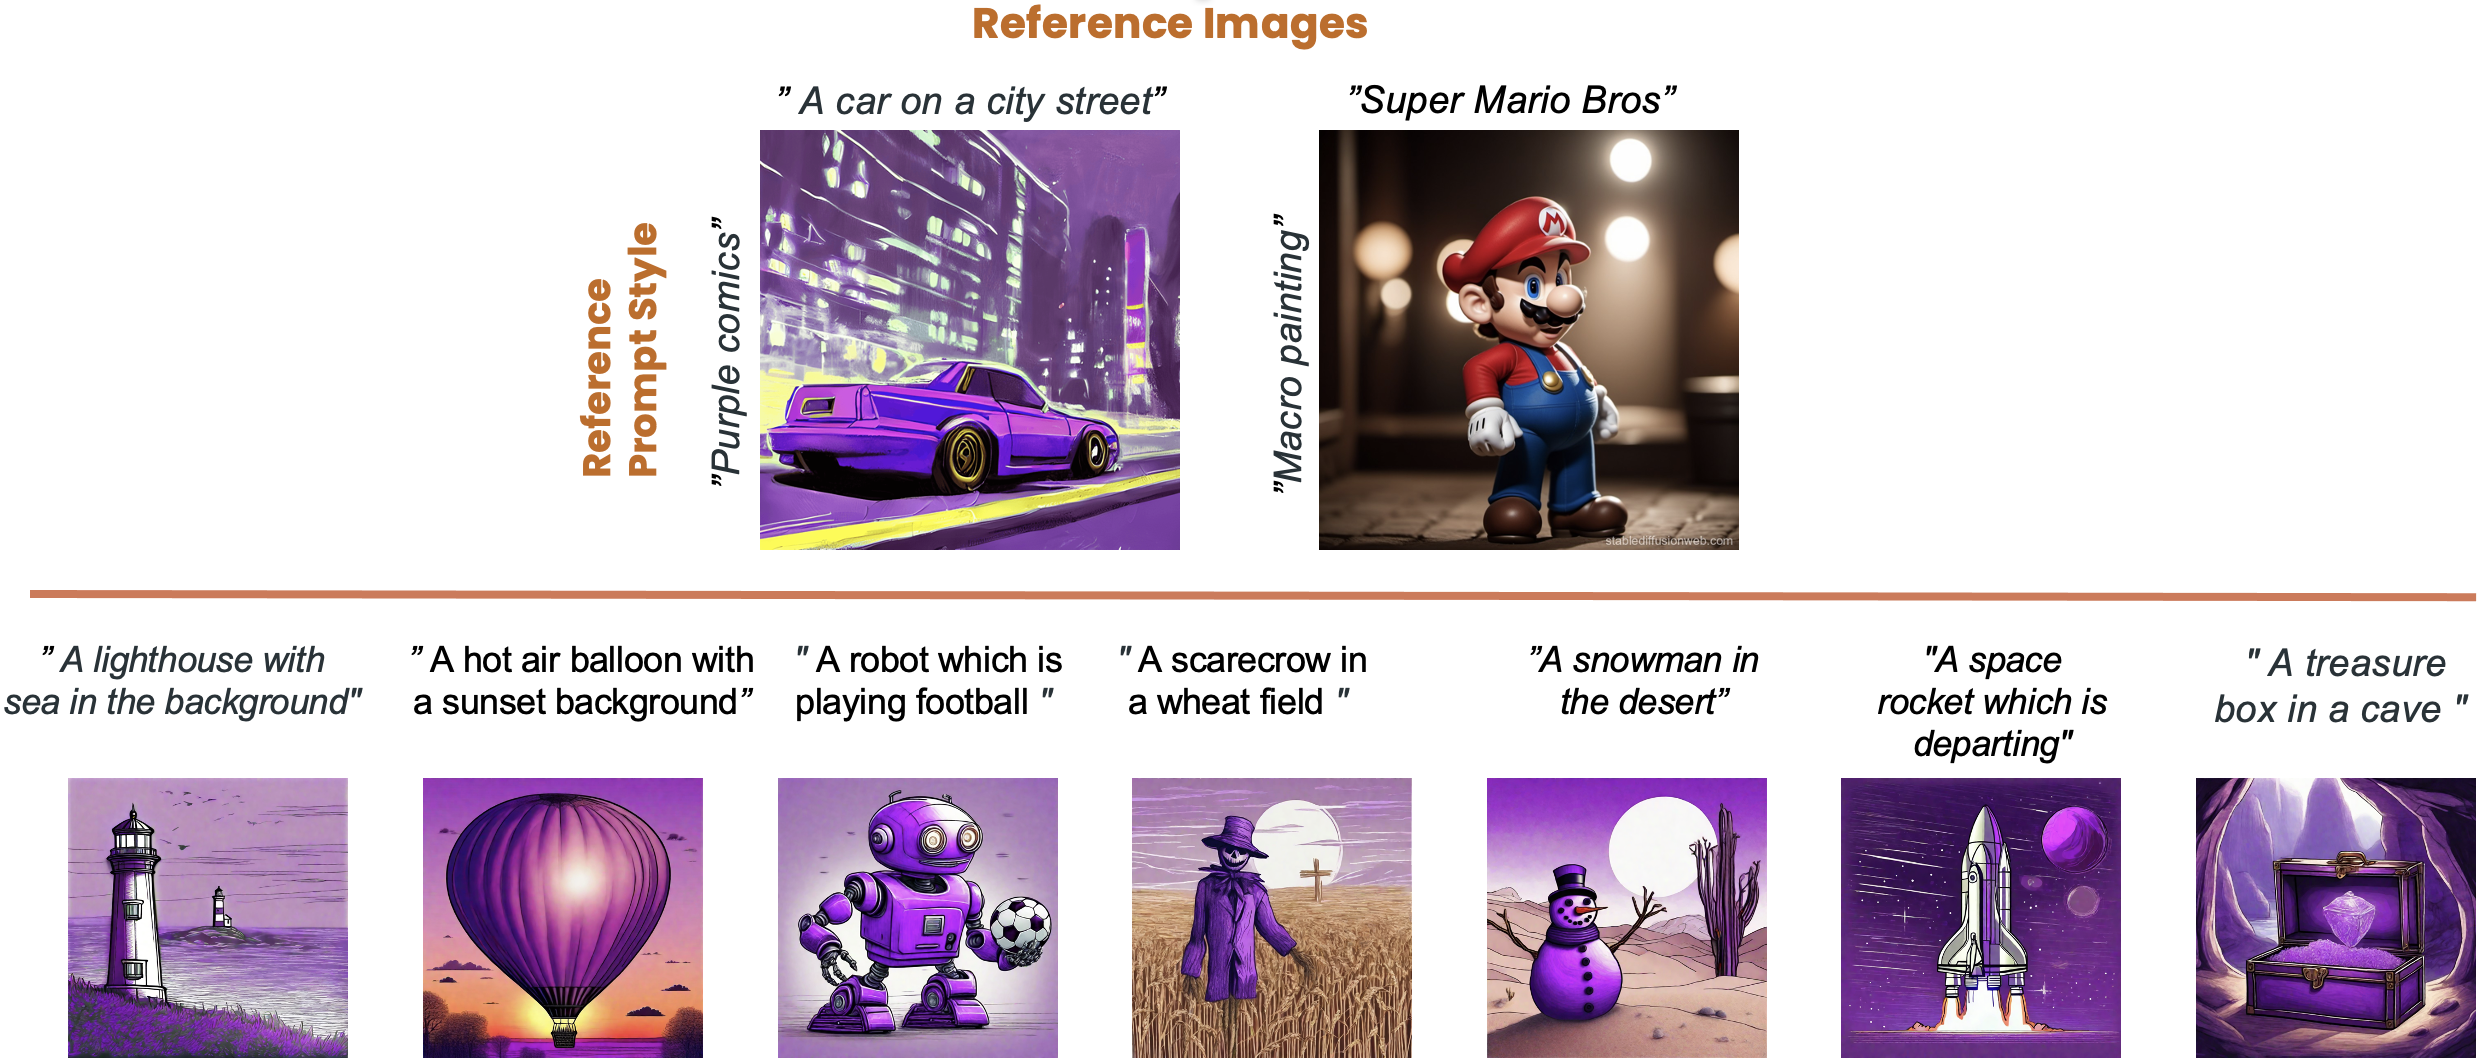}
    \caption{Purple-Comics and Macro SLI Blending (2-styles)}
    \label{blending_2_styles_purple_macro}
\end{figure*}

\begin{figure*}[ht]
    \centering
    % Second full-width image
    \includegraphics[width=\linewidth]{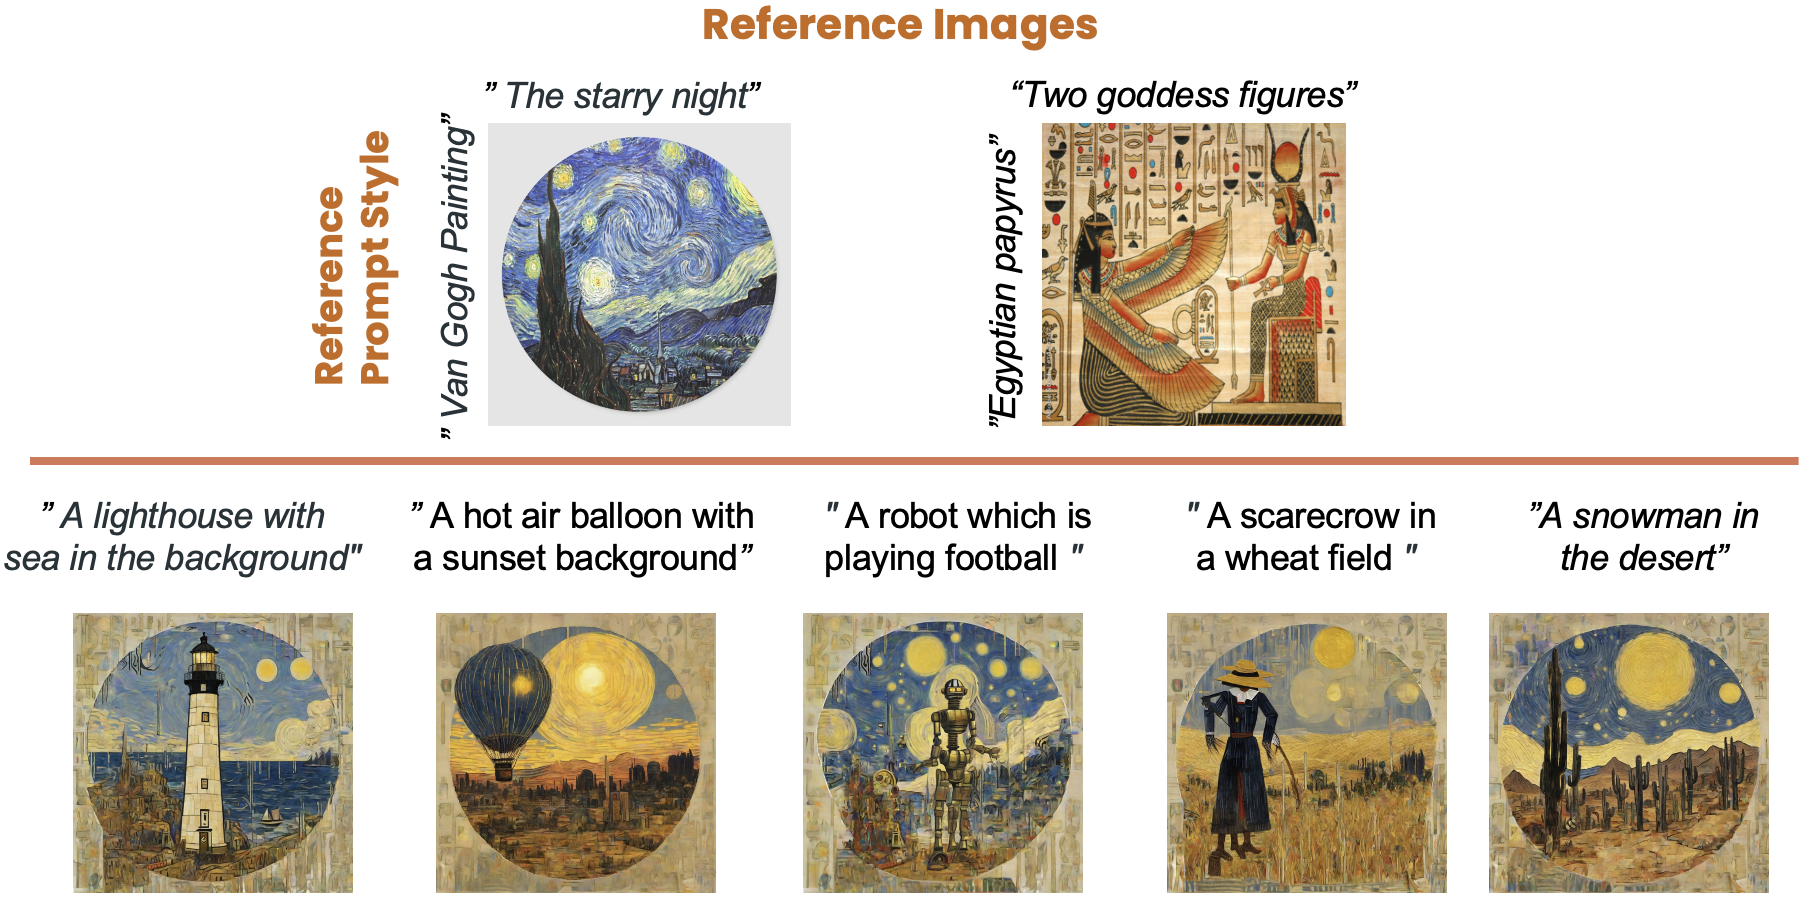}
    \caption{Van Gogh and Egyptian SLI Blending (2-styles)}
    \label{blending_2_styles_vangogh_egyptian}
\end{figure*}

\section{\textbf{Prompt List for Generated Images}}
\label{appendix:prompt_list}

Below is the list of prompts (generated with the help of ChatGPT, used for generating the images evaluated in the Weighted Multi-Style DINO VIT-B/8 experiments, used then to generate the subsets of examples  {\{$\{0, 1\}$, $\{0.15, 0.85\}$, $\{0.25, 0.75\}$, $\{0.5, 0.5\}$, $\{0.75, 0.25\}$, $\{0.85, 0.15\}$, $\{1, 0\}$\}}. Each prompt corresponds to a specific scenario in our evaluation:

\begin{itemize}
    \item \textbf{Prompt 1}: \textit{"A lighthouse with sea in the background"}
    \item \textbf{Prompt 2}: \textit{"A snowman in the desert"}
    \item \textbf{Prompt 3}: \textit{"A space rocket launching"}
    \item \textbf{Prompt 4}: \textit{"A robot playing football"}
    \item \textbf{Prompt 5}: \textit{"A scarecrow in a wheat field"}
    \item \textbf{Prompt 6}: \textit{"A mountain landscape"}
    \item \textbf{Prompt 7}: \textit{"A treasure chest in a cave"}
    \item \textbf{Prompt 8}: \textit{"A hot air balloon at sunset"}
    \item \textbf{Prompt 9}: \textit{"A castle with a flowery landscape"}
\end{itemize}

\begin{figure*}[ht]
    \centering
    \begin{minipage}[t]{0.48\linewidth}
        \centering
        % Third image (left column)
        \includegraphics[width=\linewidth]{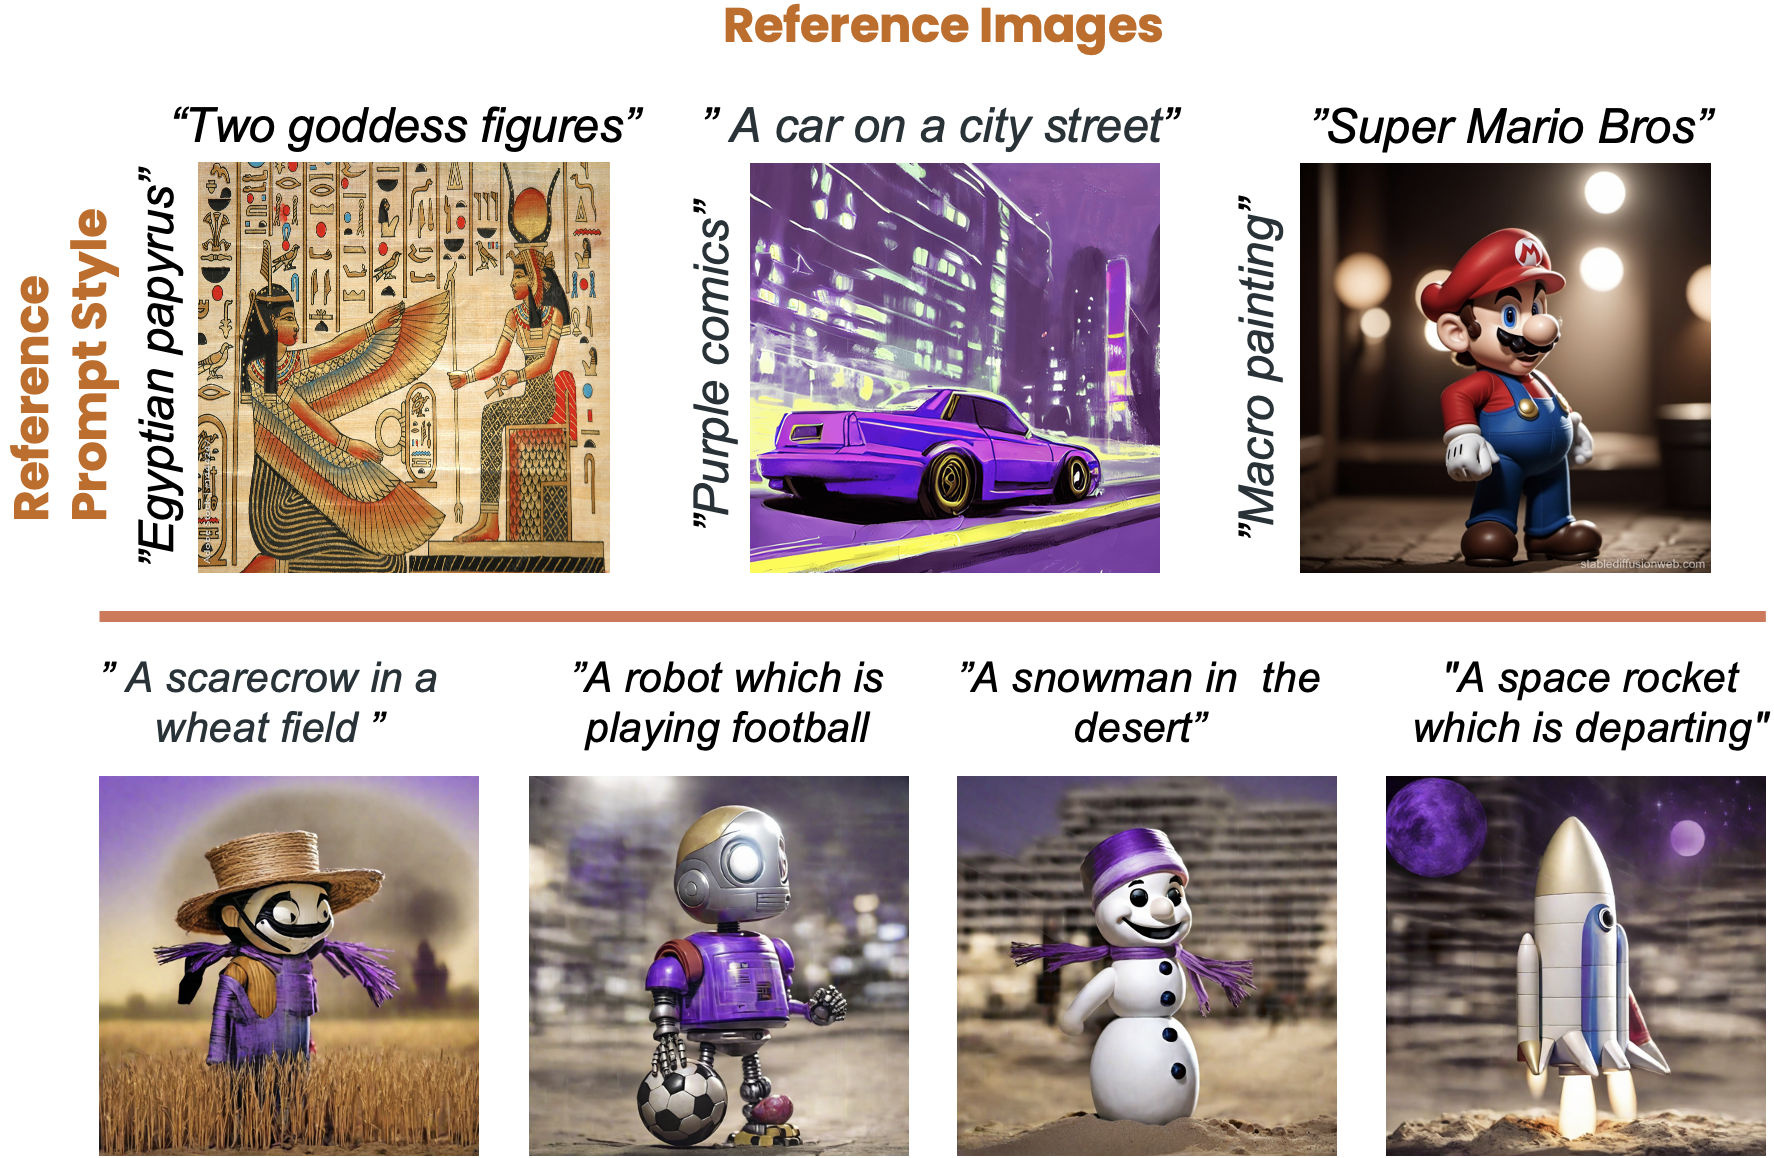}
        \caption{Egyptian, Purple-Comics, and Macro SLI Blending (3-styles)}
        \label{blending_3_styles_egyptian_purple_macro}
    \end{minipage}
    \hfill
    \begin{minipage}[t]{0.48\linewidth}
        \centering
        % Fourth image (right column)
        \includegraphics[width=\linewidth]{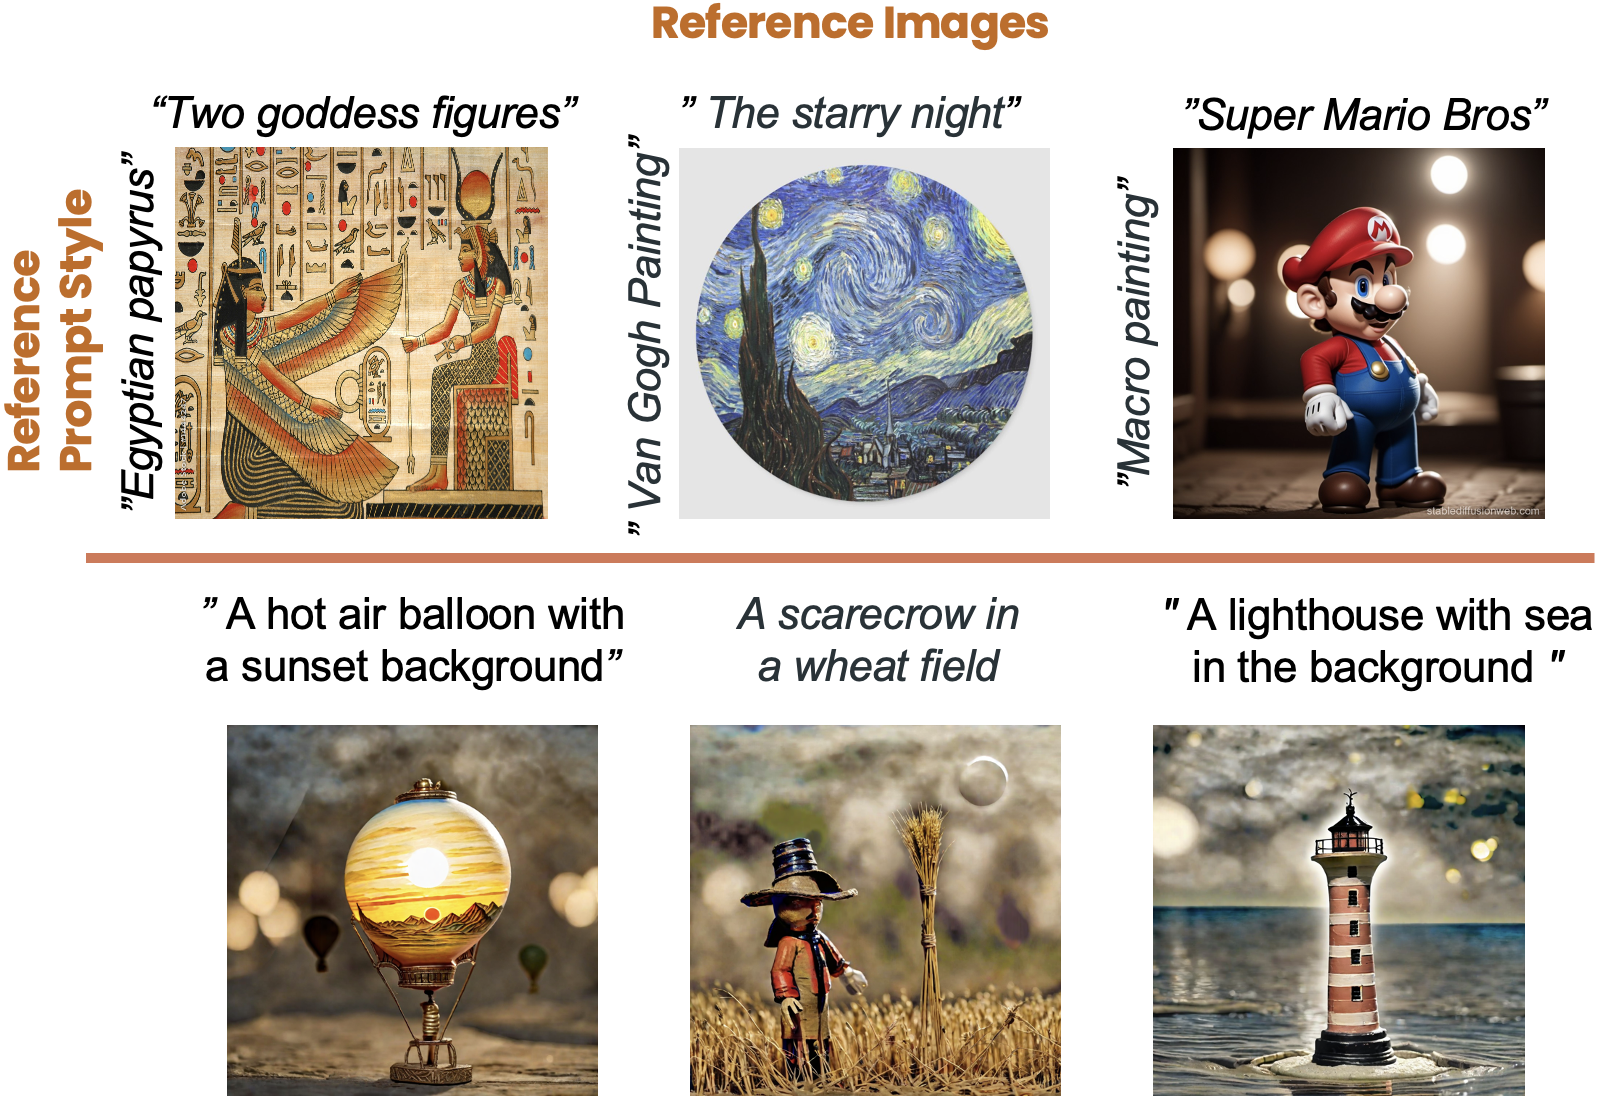}
        \caption{Egyptian, Vang Gogh, and Macro SLI Blending (3-styles)}
        \label{blending_3_styles_egyptian_vangogh_macro}
    \end{minipage}
\end{figure*}

\section{\textbf{SLI: Additional examples}}
\label{linear_slerp_additional_examples}
In this section, we provide additional qualitative examples demonstrating the application of \textbf{Spherical Linear Interpolation (SLI)} in our framework. These examples illustrate how SLI handles different style blending scenarios, emphasizing smooth transitions, feature preservation, and robustness in multi-style image generation. In \cref{blending_2_styles_purple_macro} and \cref{blending_2_styles_vangogh_egyptian} we show other examples of SLI Blending(with 0.5-0.5 weighting) maintaining style alignment in the set of generated images. In figures \cref{blending_3_styles_egyptian_purple_macro} and \cref{blending_3_styles_egyptian_vangogh_macro}, instead, we can see the same examples enriched with an additional style, making a 3 style-blending.

\section{Theoretical Justification for Multi-Style Evaluation Score Drop}
\label{WMS_scoredrop}

The Weighted Multi-Style DINO ViT-B/8 metric evaluates style consistency using cosine similarity between the embeddings of generated images and reference style embeddings, as described in \cref{subsec:wms-dino}.

\textbf{Single-Style Setting.}
In the single-style scenario, the generated image is conditioned on a single reference style image $\mathbf{s}_1$. The objective of the model is to align the image embedding $\mathbf{z}_{\text{gen}}$ as closely as possible to the reference embedding $\mathbf{z}_1$. Given the aim of maximizing style fidelity, the model tends to generate an image whose embedding is highly similar to $\mathbf{z}_1$, resulting in a high cosine similarity score.

\textbf{Multi-Style Blending Setting. }
In the multi-style setting, we aim to blend multiple reference styles $\{\mathbf{s}_1, \mathbf{s}_2, \dots, \mathbf{s}_k\}$ with corresponding weights $\{w_1, w_2, \dots, w_k\}$. The task is to generate an image whose embedding $\mathbf{z}_{\text{gen}}$ reflects a combination of these multiple-style embeddings. We compute a weighted style embedding using Linear Blending $\mathbf{z}_{\text{blend}}$ as:
\begin{equation}
    \mathbf{z}_{\text{blend}} = \sum_{i=1}^{k} w_i \mathbf{z}_i \quad 
\end{equation}
or using SLI:
\begin{equation}
    \mathbf{z}_{\text{blend}} = \text{SLI}\left(\frac{w_i}{\sum_{j=1}^{k} w_j}, \mathbf{z}_i, \mathbf{z}_j\right).
\end{equation}
The resulting blended embedding $\mathbf{z}_{\text{blend}}$ lies in the convex hull of the individual style embeddings. This implies that the generated embedding $\mathbf{z}_{\text{gen}}$ must balance between multiple style references, making it challenging to align perfectly with any single style vector.

\textbf{Why WMS$_{\text{\scriptsize DINO-ViT-B/8}}$} $<$ \textbf{DINO-ViT-B/8}.
From a geometric perspective, in the embedding space, a single vector $\mathbf{z}_{\text{gen}}$ can achieve a high cosine similarity with only one style vector $\mathbf{z}_i$ at a time. When blending multiple reference style embeddings $\{\mathbf{z}_1, \mathbf{z}_2, \dots, \mathbf{z}_k\}$, the generated embedding $\mathbf{z}_{\text{gen}}$ needs to balance its alignment across these references. This balancing act increases the angle between $\mathbf{z}_{\text{gen}}$ and any individual reference vector $\mathbf{z}_i$, reducing the cosine similarity score:
\begin{multline}
\text{CS}(\mathbf{z}_{\text{gen}}, \mathbf{z}_{\text{blend}}) < 
\max \Big(\text{CS}(\mathbf{z}_{\text{gen}}, \mathbf{z}_1), 
\\
\dots, \text{CS}(\mathbf{z}_{\text{gen}}, \mathbf{z}_k)\Big).
\end{multline}
The blended style vector $\mathbf{z}_{\text{blend}}$ introduces a divergence from any single style reference due to the averaging effect inherent in multi-style blending. This divergence results in a lower cosine similarity score in the multi-style setting.

\begin{figure*}[t]
    \centering
    \includegraphics[width=\textwidth]{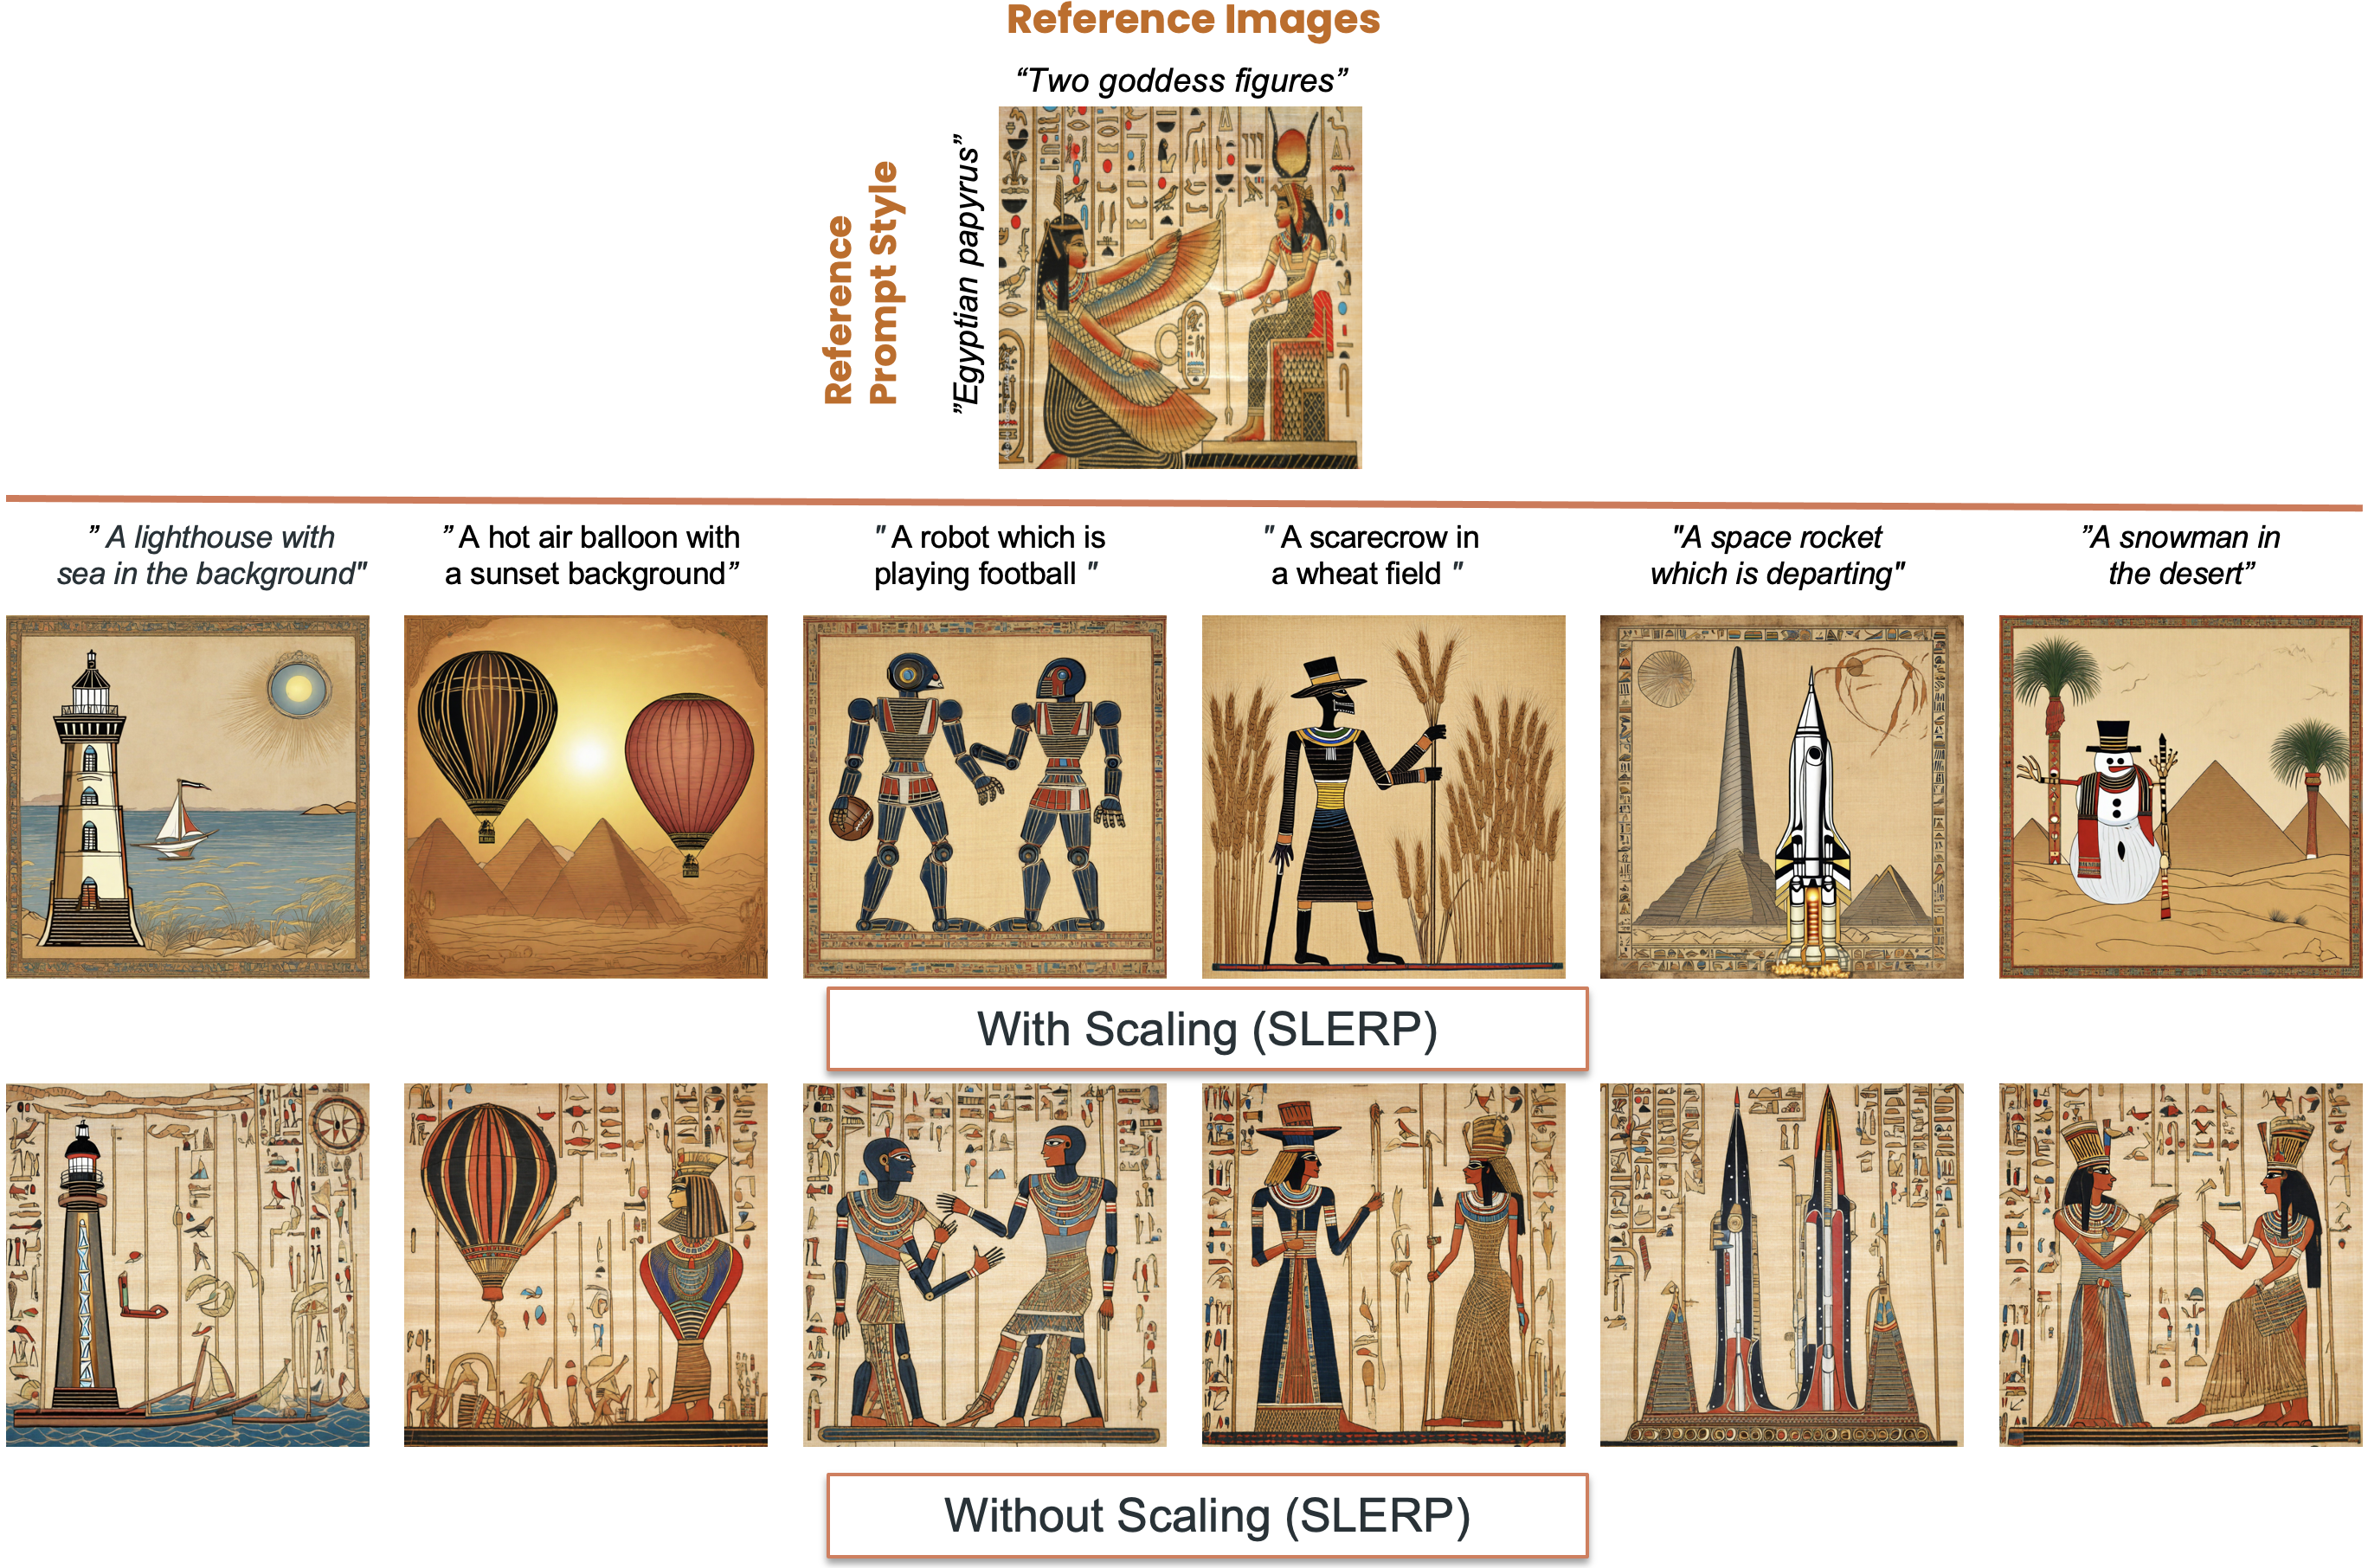}
    \caption{Attention Rescaling: Famous Image (Papyrus)}
    \label{egyptian_rescaling}
\end{figure*}
\section{\textbf{Attention Rescaling: Necessity and Theoretical Justification}}
\label{appendix:attention_rescaling}

\begin{figure}[h]
\centering
\includegraphics[width=\linewidth]{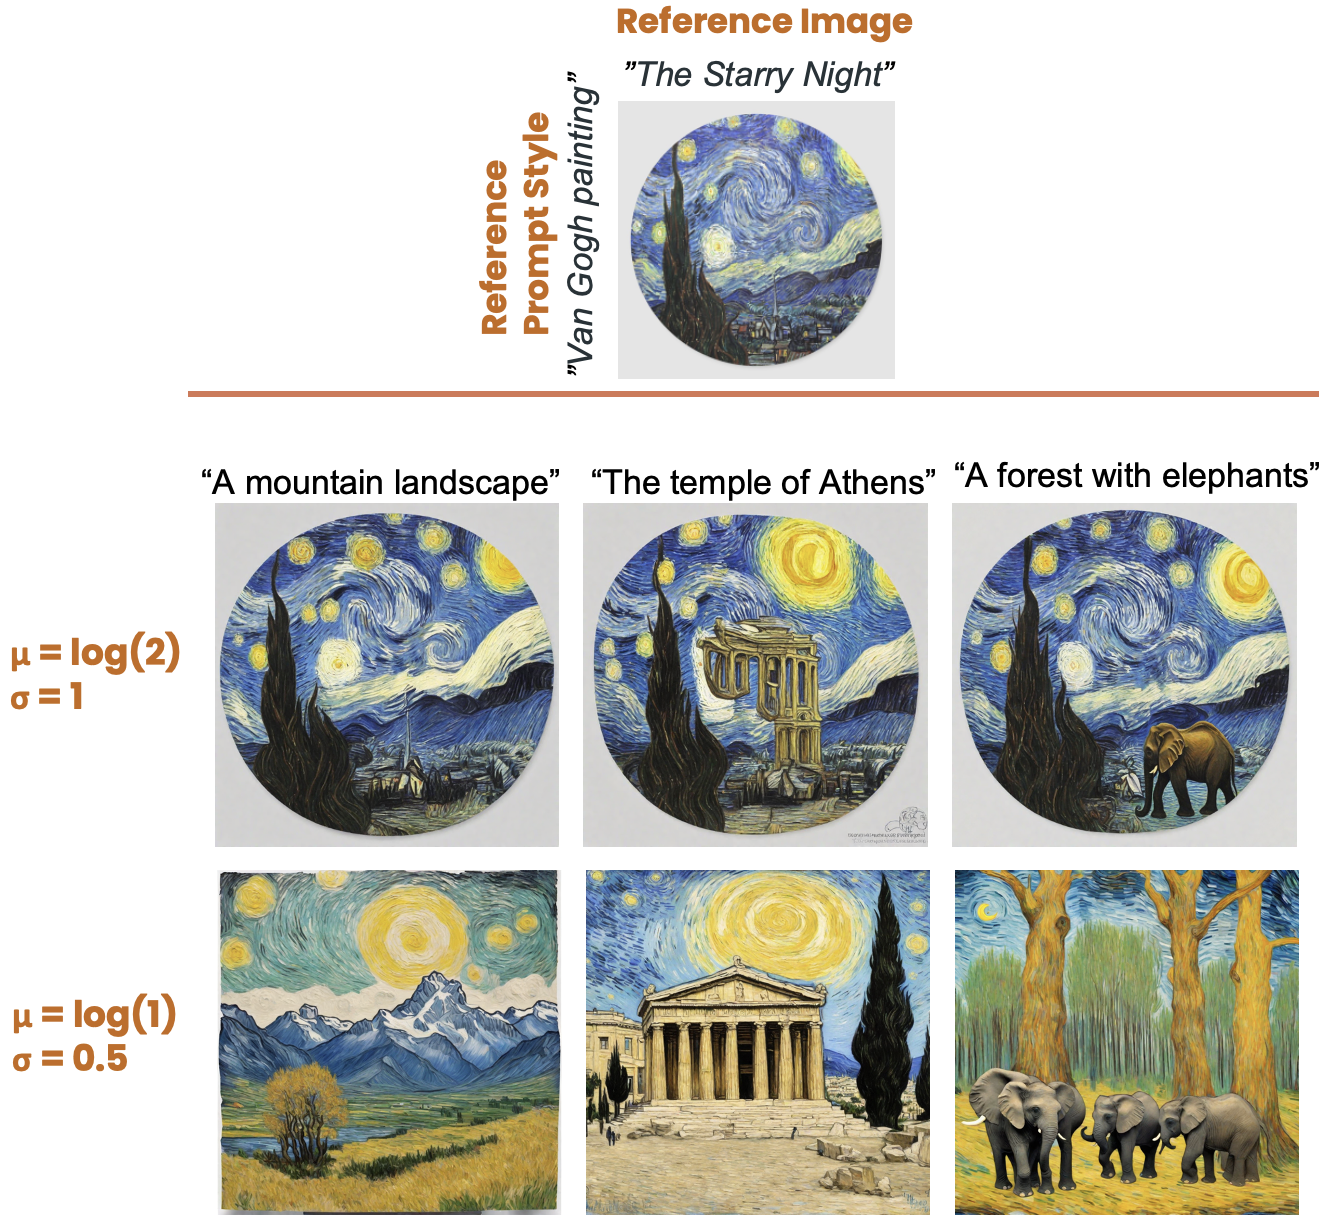}
\caption{Attention Rescaling: Famous Image (Van Gogh)}
\label{vangogh_rescaling}
\end{figure}

\textbf{Key Insight.}
Cosine similarity measures the alignment between vectors, and achieving high alignment with multiple style vectors simultaneously is mathematically infeasible unless the vectors are collinear (perfectly aligned), which is unlikely in a complex style embedding space. Thus, the Weighted Multi-Style DINO ViT-B/8 score in the multi-style setting cannot exceed, and will generally be lower than, the score in a single-style setting due to the fundamental properties of vector space geometry and cosine similarity.

This decrease in the metric score is not a flaw of the evaluation process but rather a reflection of the increased complexity and trade-offs in generating images that incorporate multiple stylistic influences. It highlights the challenge of achieving stylistic coherence when multiple, diverse style references are used, underscoring the importance of our novel blending techniques that aim to mitigate this inevitable drop in alignment quality.

In generative models like Stable Diffusion, attention mechanisms play a pivotal role in aligning the generated content with the style conditioning input. However, when extending the work from Hertz \etal \cite{hertz2023StyleAligned} framework to incorporate multi-reference style blending, the standard attention mechanisms require modification to handle the increased complexity. Here, we introduce the concept of Attention Rescaling, which addresses two main issues: style dominance and multi-style consistency.

\textbf{Style Dominance Problem.} In the context of conditioning with multiple style references, the generated image's features are influenced by multiple style embeddings. Without rescaling, the attention weights can become biased towards the dominant style vector, especially when the styles have varying degrees of prominence in the latent space. Let \( A_i \) denote the attention weight for the \(i\)-th style reference and \(\mathbf{z}_i\) be its corresponding latent vector. The unscaled attention score is computed as:
\begin{equation}
    \text{Attention}(Q, K_i) = \frac{Q \cdot K_i^\top}{\sqrt{d}}
\end{equation}
where \(Q\) is the query feature, \(K_i\) is the key feature of the \(i\)-th style reference, and \(d\) is the dimensionality of the latent space.

When multiple style references are used, the total attention weight becomes:
\begin{equation}
    A_{\text{tot}} = \sum_{i=1}^{k} A_i = \sum_{i=1}^{k} \frac{\exp(\text{Attention}(Q, K_i))}{\sum_{j=1}^{k} \exp(\text{Attention}(Q, K_j))}
\end{equation}
In practice, this can lead to an imbalance where one style overly influences the generation process, diminishing the contributions of other styles.

\textbf{Attention Rescaling Solution.} To mitigate this issue, we apply Attention Rescaling by introducing a normalization factor \(\lambda_i\) for each style reference. The rescaled attention score is given by:
\begin{equation}
    \text{Rescaled Attention}(Q, K_i) = \frac{\lambda_i (Q \cdot K_i^\top)}{\sqrt{d}}
\end{equation}
The normalization factor \(\lambda_i\) is computed based on the relative weight \(w_i\) of each style, ensuring that the contribution of each style is proportional to its intended influence:
\begin{equation}
    \lambda_i = \frac{w_i}{\sum_{j=1}^{k} w_j}
\end{equation}
This adjustment redistributes the attention across all style references, preventing any single style from dominating the blending process and ensuring a balanced influence. After the rescaling, we can observe a certain degree of diversity in the generation of the images. An example of the solution can be observed in \cref{egyptian_rescaling} where, without attention rescaling, the images present almost the same details, making the content of the generated images take a back seat. Another example is shown in \cref{vangogh_rescaling} where the famous image ("The Starry Night"), influences too much the generation, producing almost identical images.

\textbf{Impact on Style Blending.} We empirically observe that Attention Rescaling enhances the quality of style blending, particularly in high-dimensional latent spaces. Without rescaling, the generated images often exhibit artifacts or an over-representation of one style. With rescaling, the transition between styles is smoother, and the blended image retains a balanced representation of all reference styles. This approach is particularly beneficial when using SLI for latent space interpolation, as it ensures that the geometric properties of the styles are respected during the blending process.

\begin{figure*}[htbp]
    \centering
    \begin{minipage}[t]{0.48\linewidth}
        \centering
        \includegraphics[width=\linewidth]{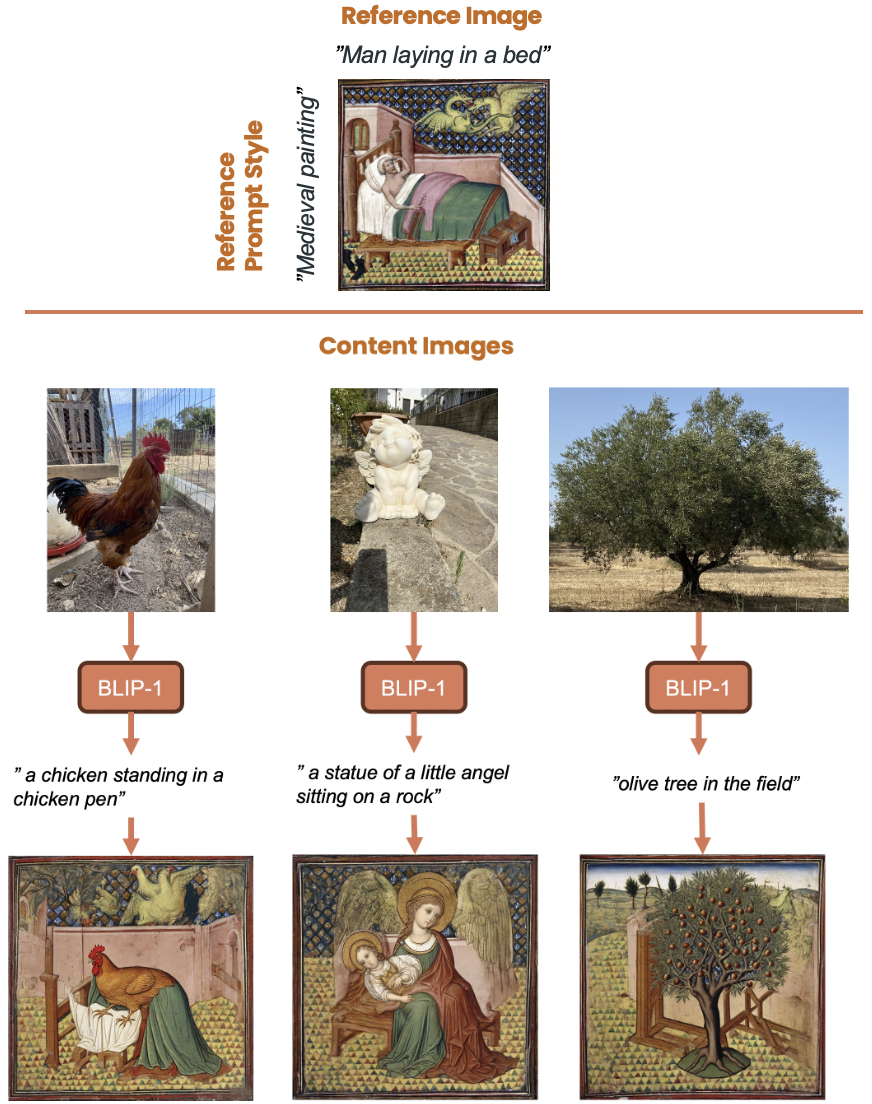}
        \caption{Image-to-Text: Image generation with style alignment based on Image Content.}
        \label{fig:img_mode}
    \end{minipage}
    \hfill
    \begin{minipage}[t]{0.48\linewidth}
        \centering
        \includegraphics[width=\linewidth]{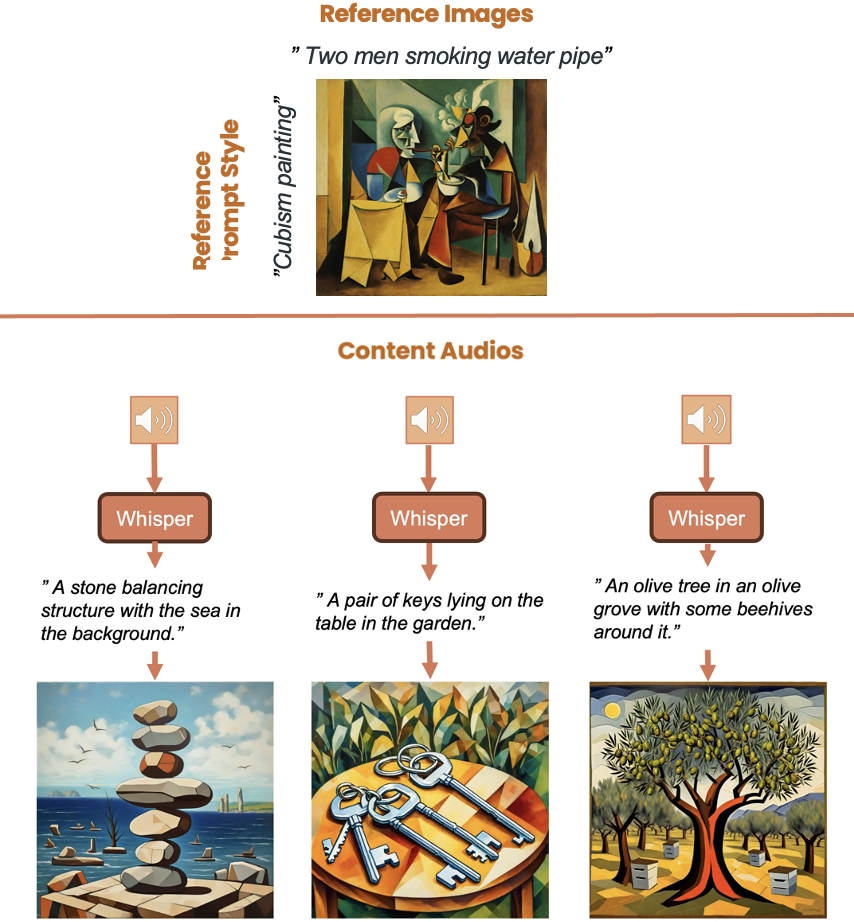}
        \caption{Audio-to-Text: Image generation with style alignment based on Audio Content.}
        \label{fig:audio_mode}
    \end{minipage}
\end{figure*}

\section{\textbf{Additional Examples of Multi-Modal Content Fusion}}
\label{appendix:multi_modal_examples}

In this section, we provide additional qualitative examples demonstrating the effectiveness of our Multi-Modal Content Fusion pipeline. We present results for different input modes, including image-based content, audio-based content, music-based content, environmental data-based content, as well as various combinations of these inputs. 

\subsection{\textbf{Single-Mode Examples}}
\label{appendix:single-mode}

In \cref{fig:img_mode}, we can observe the image generation results, with style alignment, we obtain when providing contextual information through images. In \cref{fig:audio_mode}, instead, we can notice the image generation results, with style alignment, but with audio contextual information.

% Full-width image (first row)
\begin{figure*}[htbp]
    \centering
    \includegraphics[width=\textwidth]{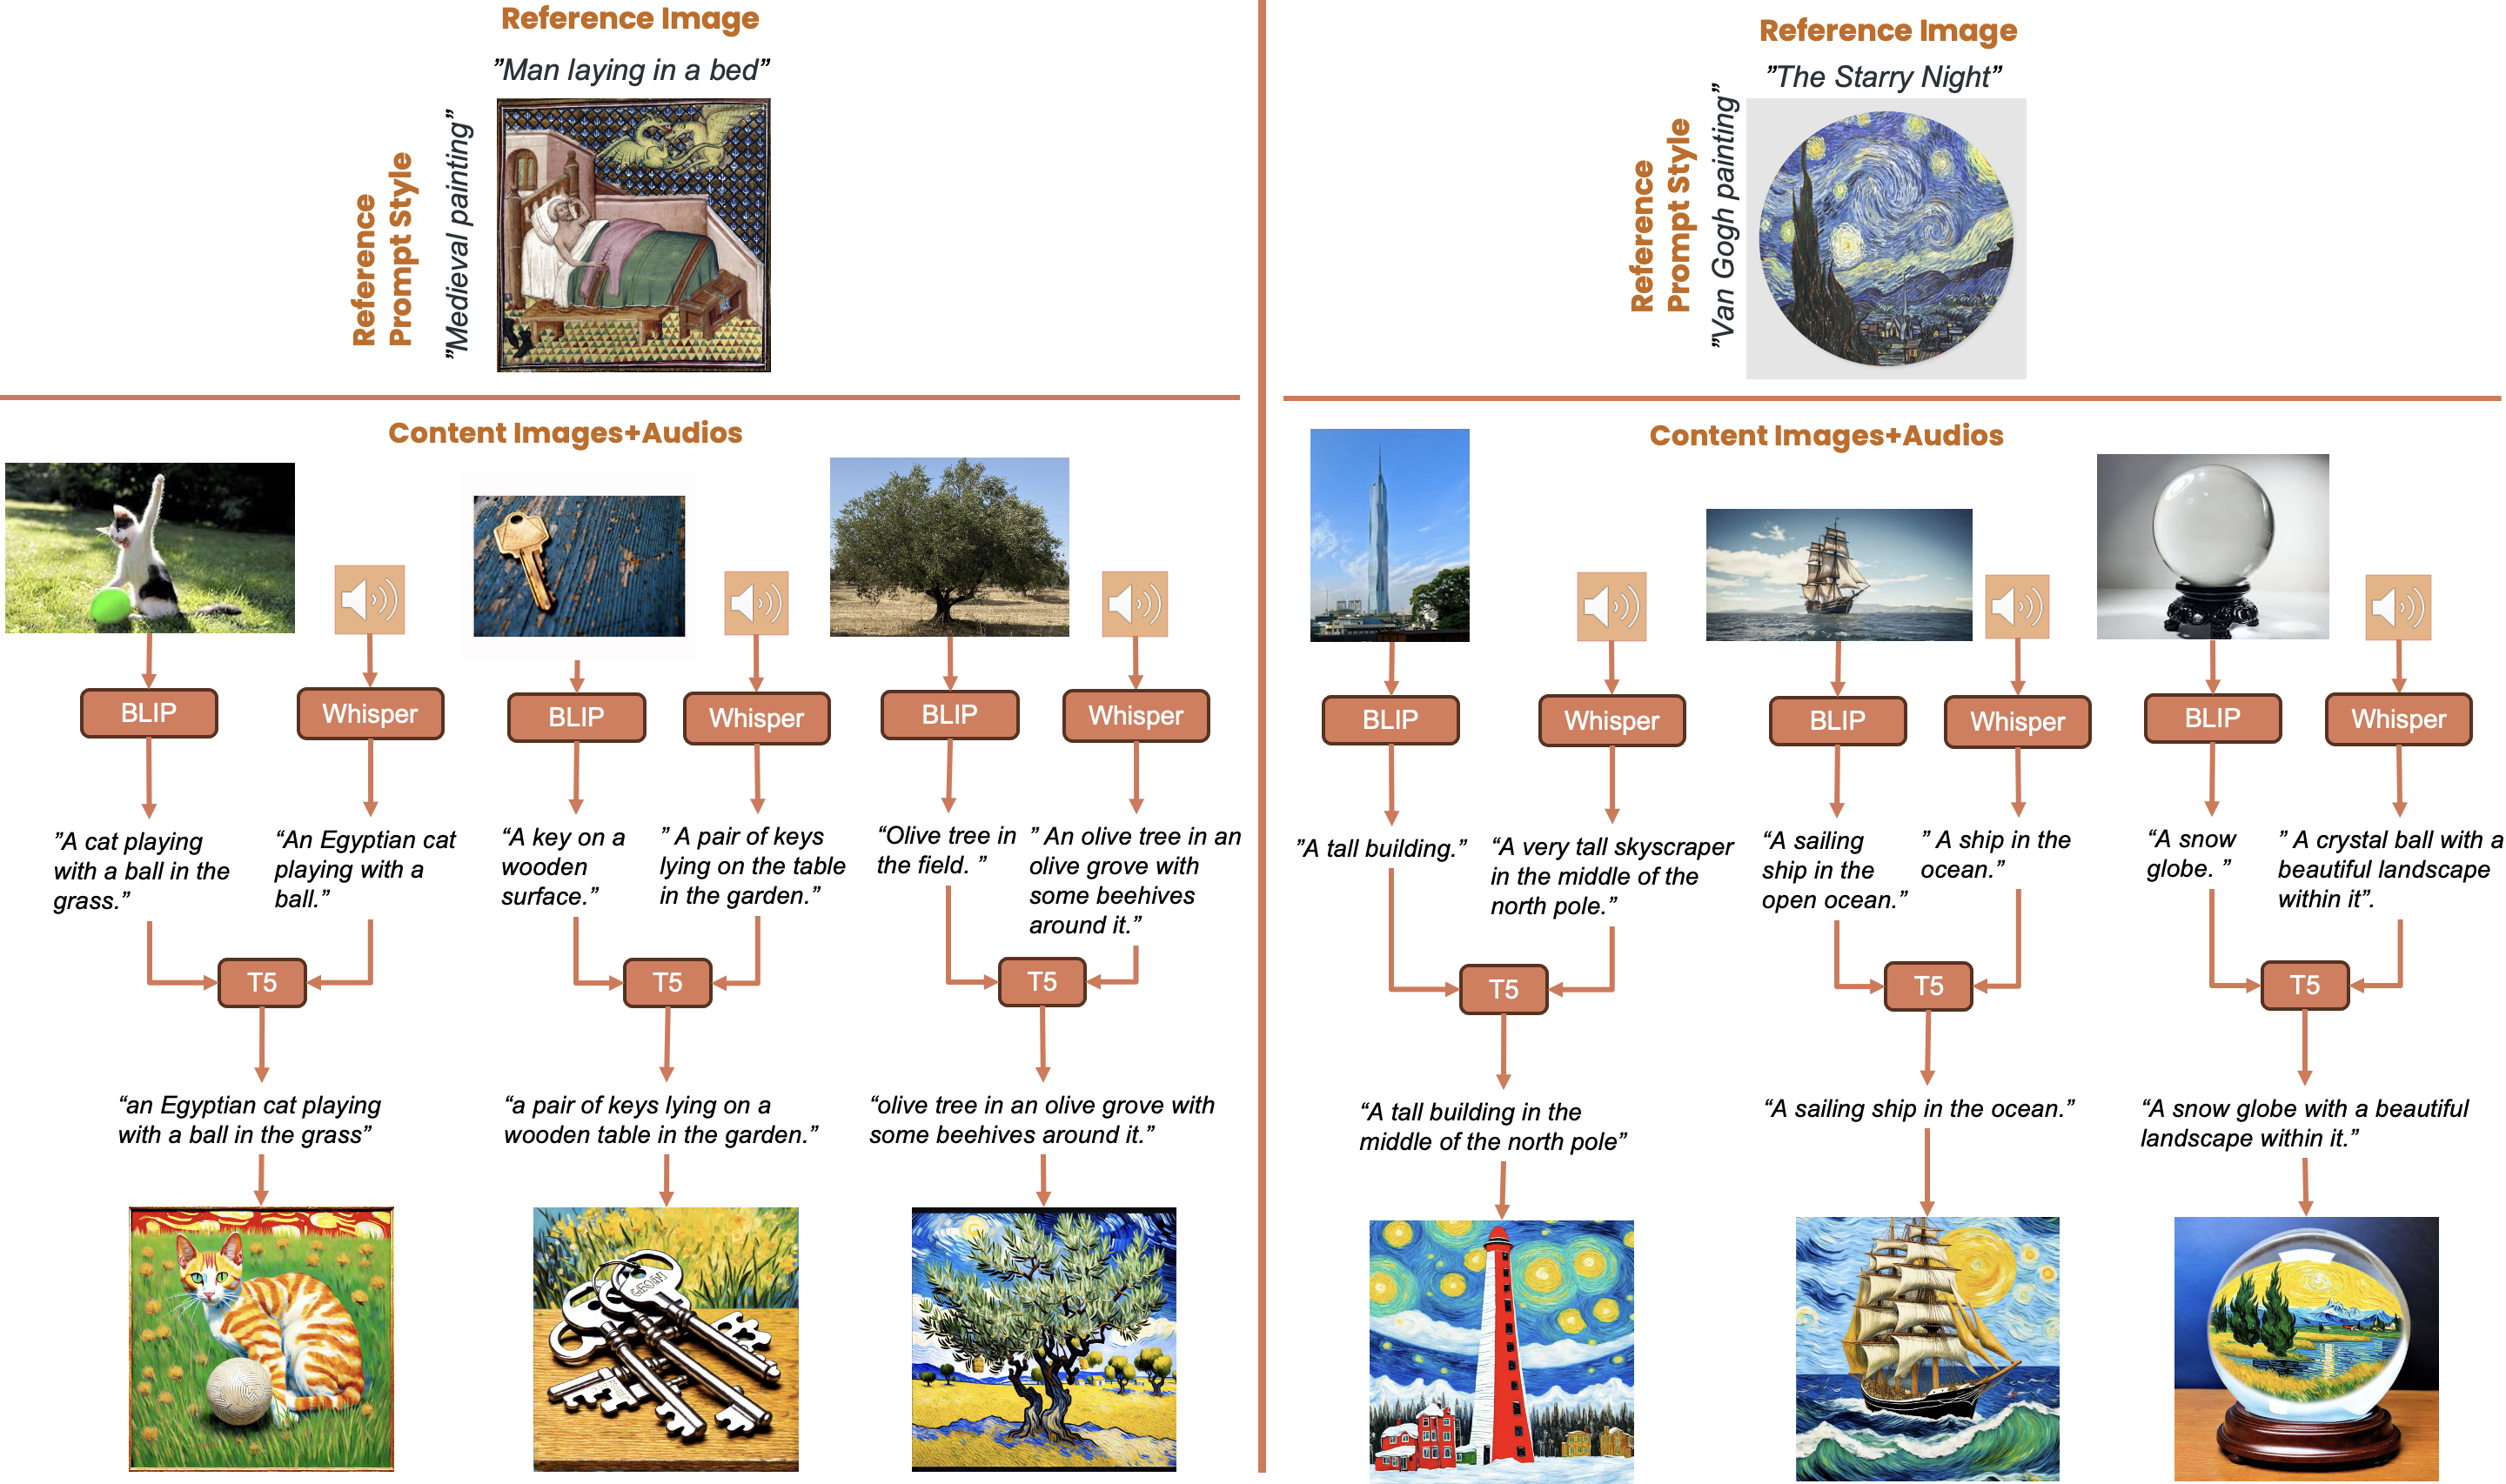}
    \caption{Image-to-Text + Audio-to-Text: Two examples of image generation with style alignment based on both image and audio contextual information.}
    \label{img_audio_mode_examples}
\end{figure*}

% Side-by-side images (second row)
\begin{figure*}[htbp]
    \centering
    \begin{minipage}[t]{0.48\linewidth}
        \centering
        \includegraphics[width=\linewidth]{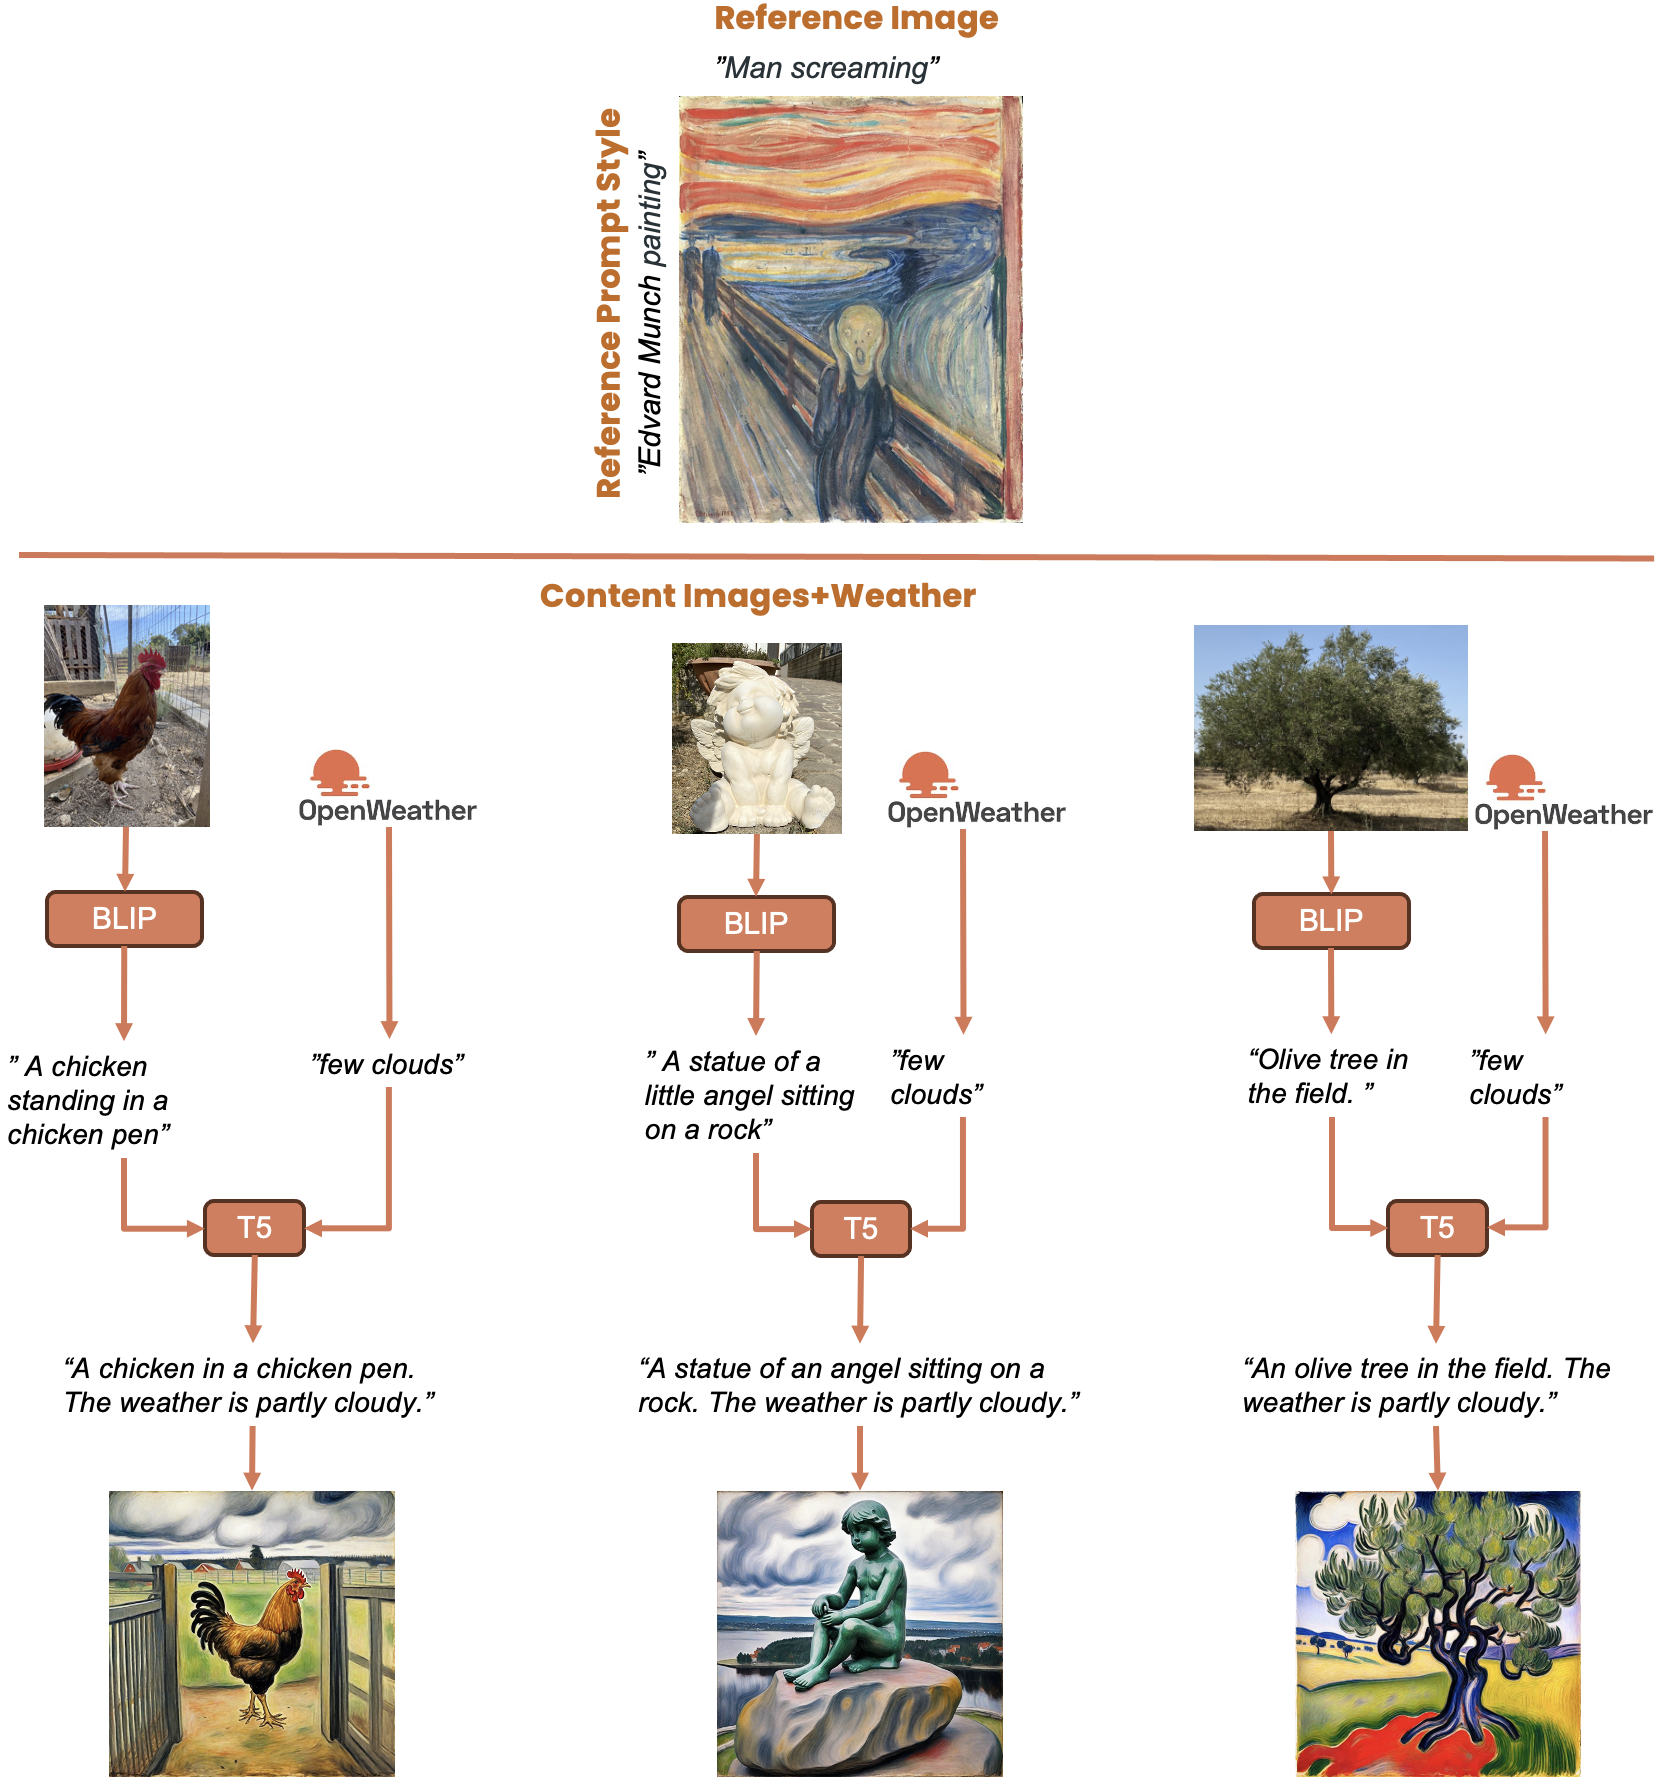}
        \caption{Image-to-Text + Weather-to-Text: Image generation with style alignment based on both image and weather contextual information.}
        \label{img_weather_mode}
    \end{minipage}
    \hfill
    \begin{minipage}[t]{0.48\linewidth}
        \centering
        \includegraphics[width=\linewidth]{figures/Appendix/Content/Images_Weather_Mode.png}
        \caption{Image-to-Text + Weather-to-Text Ablation: Image generation with style alignment based on image and weather contextual information, highlighting style blending differences.}
        \label{img_weather_ablation_mode}
    \end{minipage}
\end{figure*}

% Side-by-side images (third row)
\begin{figure*}[htbp]
    \centering
    \begin{minipage}[t]{0.48\linewidth}
        \centering
        \includegraphics[width=\linewidth]{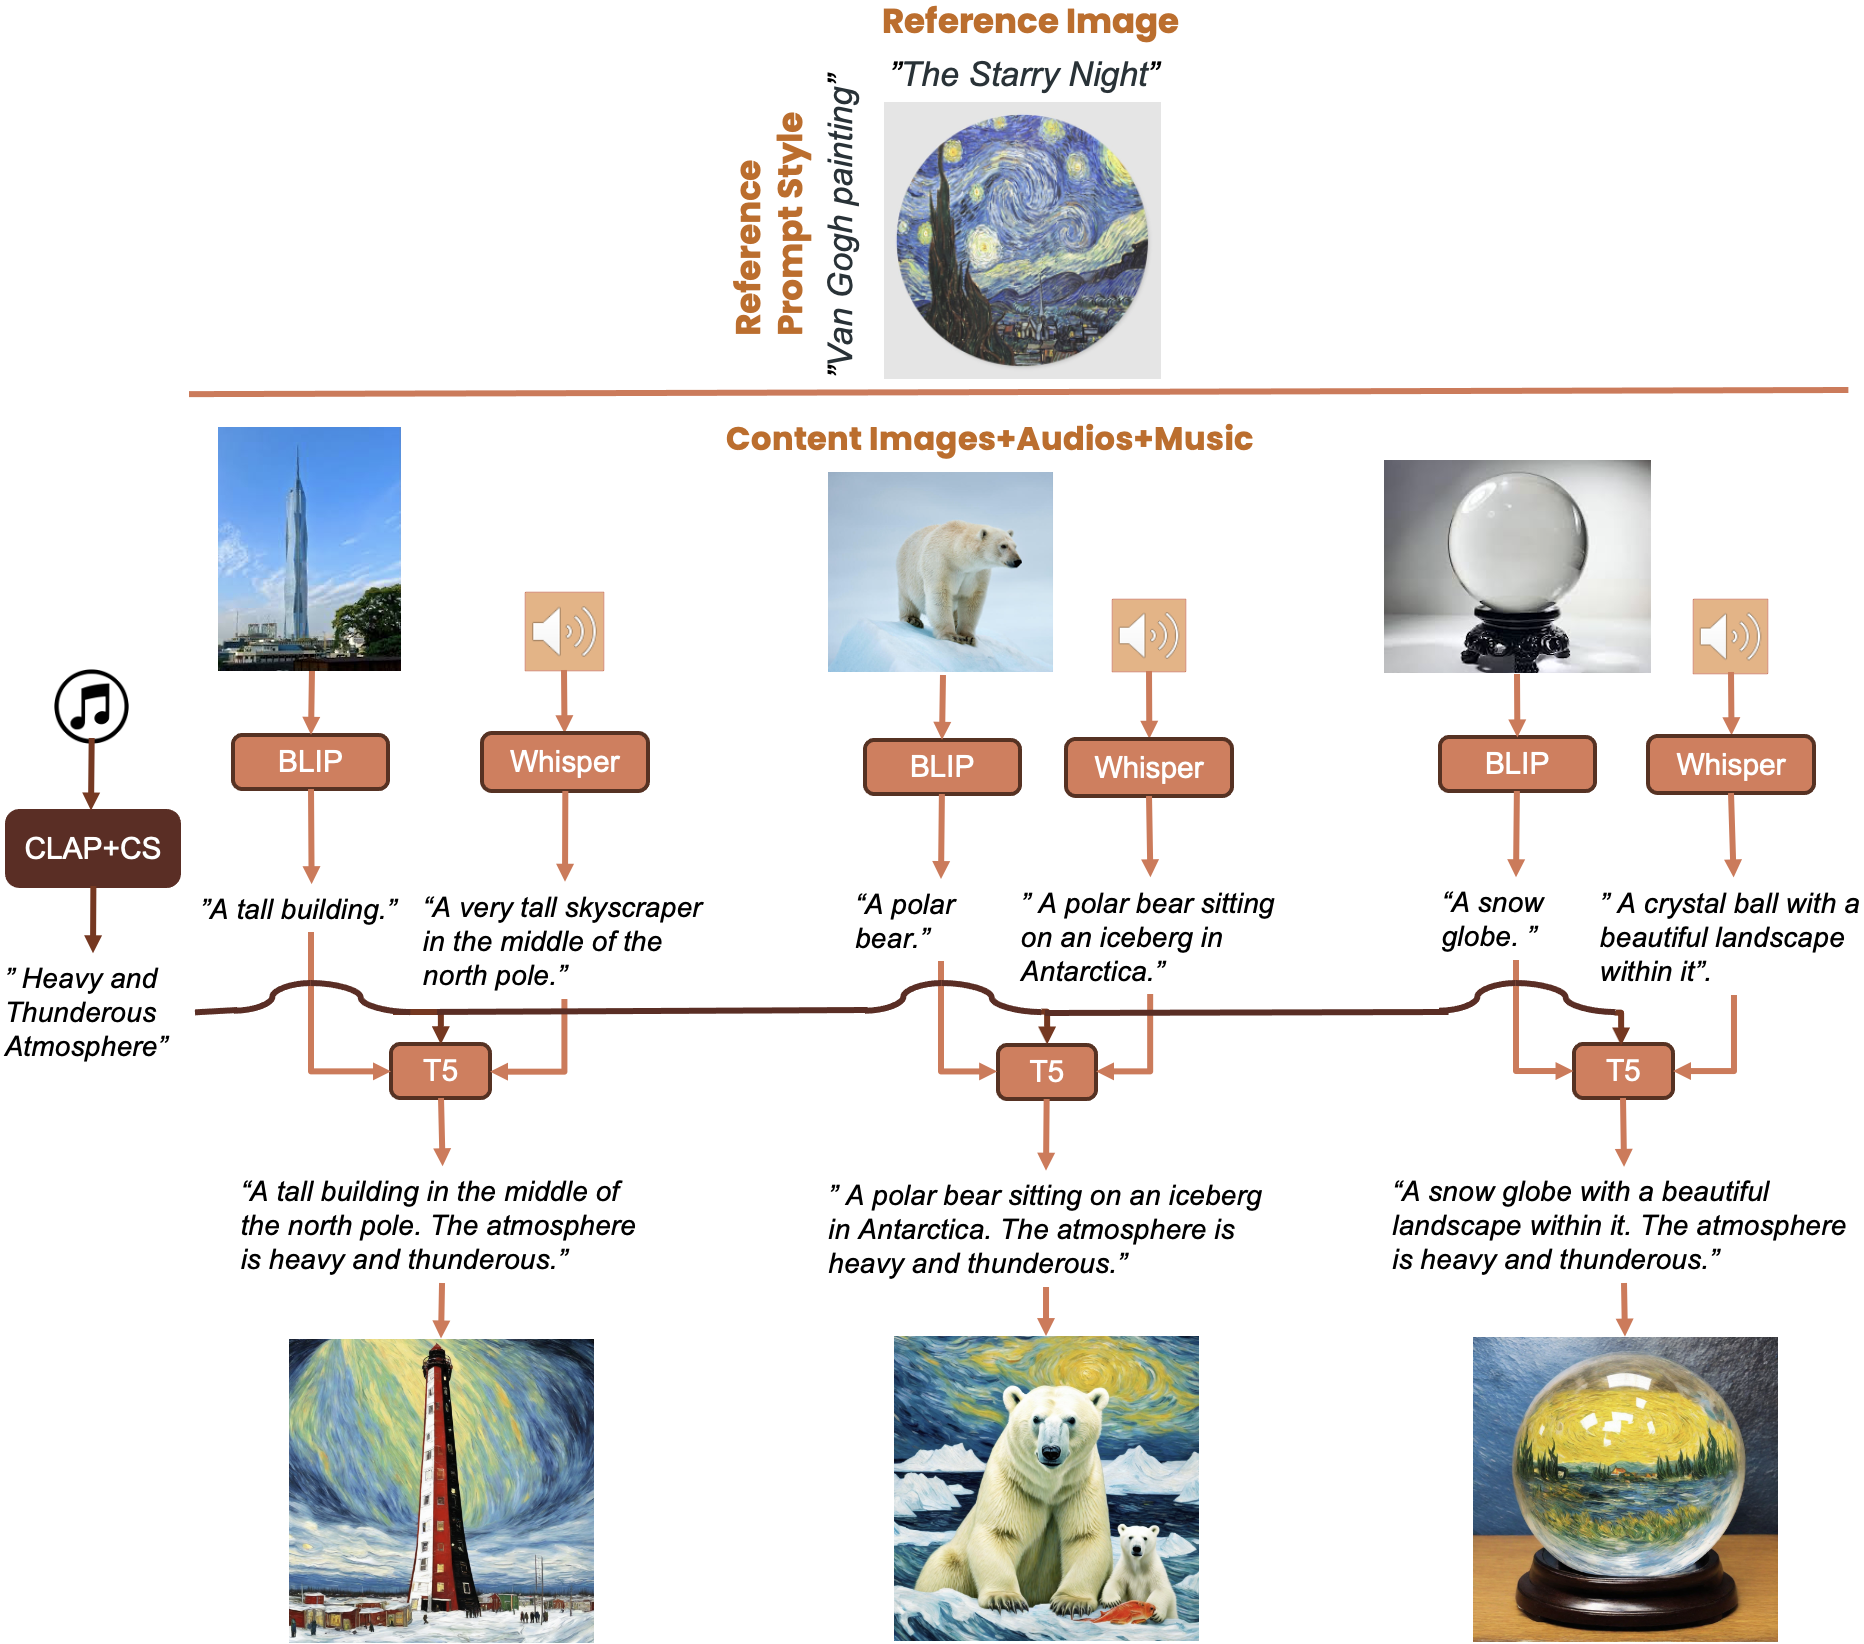}
        \caption{Image-to-Text + Audio-to-Text + Music-to-Text Ablation: Image generation with style alignment based on image, audio, and music contextual information.}
        \label{img_audio_music_mode}
    \end{minipage}
    \hfill
    \begin{minipage}[t]{0.48\linewidth}
        \centering
        \includegraphics[width=\linewidth]{figures/Appendix/Guidance_Ablation.png}
        \caption{SLI: Guidance Ablation showing the effect of different guidance scaling factors.}
        \label{slerp_guidance_ablation_imgs}
    \end{minipage}
\end{figure*}

\subsection{\textbf{Multi-Modal Fusion Examples}}
\label{appendix:multi_modal_fusion}

Finally, we demonstrate the results when combining multiple input modalities, showcasing the capability of our framework to integrate diverse sources of content information. In particular, in \cref{img_audio_mode_examples}, we can see two examples of a bi-modal fusion, in which we are given contextual information both through image and audio modality. Here, they are then merged into the rephrasing step, ending with the generation of bi-modal style-aligned images. Another example of bi-modality we present is in \cref{img_weather_mode}, where the contextual information comes from both the image and the weather information. In \cref{img_weather_ablation_mode}, we make an ablation depending on different weather conditions we could have. A last example presented for this section provides a tri-modal fusion, in \cref{img_audio_music_mode}, in which we present a content fusion based on the image, audio, and music modalities.

\section{\textbf{SLI Guidance Ablation: Additional Results}}
\label{appendix:slerpguidance_ablation}

In this section, we provide additional qualitative results from our ablation study on SLI Guidance, analyzing its impact on multi-style blending and image generation quality. The experiments are conducted using different configurations of SLI, varying the interpolation weights and guidance strength to assess their effects on style coherence and feature preservation. Some qualitative results can be observed in \cref{slerp_guidance_ablation_imgs}, where it is shown how the set of generated images changes depending on the guidance choice.
